# Supplementary material for: Is Pseudo-Lidar needed for Monocular 3D Object detection?
Source: arXiv:2108.06417 source file (2021-08-13)
Supplement: Supplementary file 1 [file suppmat.tex]

\section{Introduction}
The goal of this supplementary document is to provide additional details complementing our main paper: detailed Pseudo-Lidar results - Section~\ref{sec:pretraining_detailed}; detailed nuScenes~\cite{caesar2020nuscenes} results - Section~\ref{sec:nusc_detailed}; Cityscapes3D~\cite{gahlert2020cityscapes} results - Section~\ref{sec:cityscapes}; detailed DD3D fine-tuning results - Section~\ref{sec:fcos_ablative}; depth pre-training schedule - Section~\ref{sec:pretraining}; Pseudo-Lidar 3D confidence head implementation details - Section~\ref{sec:pl_detection_head}; DD3D architecture details - Section~\ref{sec:fcos_architecture}; qualitative results - Section~\ref{sec:qualitative}.

% on (i) the experimental results presented in the main paper that were omitted due to lack of space and (ii) the architectures and training setup of the FCOS-3D and Pseudo-Lidar approaches to facilitate the reproduction of our results.

\section{Pseudo-Lidar detailed results}
\label{sec:pretraining_detailed}

% We pre-train our monocular depth estimator PackNet~\cite{guizilini20203d} on 4 splits (\textit{1K}, \textit{5K}, \textit{10K}, \textit{25K}), as well as starting from scratch. Following this pre-training stage, we fine-tune the depth estimator on the KITTI3D~\cite{geiger2012we} \textit{Eigen clean} depth split. Finally, for each depth model we train a Pseudo-Lidar 3D detector using the KITTI3D train split.
In this section we present detailed depth and 3D detection results, complementing the summary presented in Fig. 4 in the main submission. These results are summarized in Table~\ref{table:supp_pl_data_vs_det}, where we note the trend of improving with data for both the depth and the 3D detection results, as well as the correlation between the two.

\begin{table}[h!]
\centering
{
\footnotesize
\setlength{\tabcolsep}{0.5em}
\rowcolors{2}{lightgray}{white}
\begin{tabular}{l|ccc|ccc}
\toprule
& \multicolumn{3}{c}{Data split} & \multicolumn{3}{c}{3D AP} \\ 
\multirow{-2}{*}{Depth net} & 
Abs Rel$\downarrow$ &
Sq Rel$\downarrow$ &
RMSE$\downarrow$&
Easy$\uparrow$ & Med$\uparrow$ & Hard$\uparrow$ \vspace{0.5mm}\\
\midrule

\textbf{Scratch}  & 
0.112 & 
0.761 &  
4.756 &  
18.11 &  
12.70 &  
10.63 \\

 \textbf{1K}  & 
0.101 & 
0.560 &  
3.891 &  
22.13 &  
15.05 &  
13.00 \\

\textbf{5K}  & 
0.093 & 
0.505 &  
3.692 &  
28.86 &  
18.88 &  
15.67 \\

\textbf{10K}  & 
0.091 & 
0.501 &  
3.722 &  
27.35 &  
18.41 &  
15.25 \\

\textbf{25K}  & 
0.079 & 
0.489 &  
3.577 &  
32.10 &  
22.36 &  
19.20 \\

\bottomrule
\end{tabular}\\\vspace{0mm}
\caption{
%\textbf{3D detection accuracy on the KITTI3D~\cite{geiger2012we} validation split with different depth inputs.} 
\textbf{How accurate does the depth predictor need to be for the Pseudo-Lidar detector?} We train a PackNet~\cite{guizilini20203d} depth estimator with increasing amounts of training data, subsequently fine-tuned on the KITTI3D Eigen clean split. We generate depth maps from each depth network on the KITTI3D train and validation splits, and train a Pseudo-Lidar 3D detector using predicted depth as input. We report $AP|_{40}$ metric on the \textit{Car} class. Both 3D and depth metrics are computed on the KITTI3D \emph{val} set. Note that this table complements Fig. 4 in the main paper.}
\label{table:supp_pl_data_vs_det}
}
\end{table}

\section{nuScenes~\cite{caesar2020nuscenes} detailed results}
\label{sec:nusc_detailed}

\begin{table}[!h]
\centering
{
\footnotesize
\setlength{\tabcolsep}{1em}
\rowcolors{2}{lightgray}{white}
\begin{tabular}{l|cccc}
\toprule
& \multicolumn{4}{c}{AP [\%] $\uparrow$} \\

\multirow{-2}{*}{Category}& 
0.5m & 1.0m & 2.0m & 4.0m \vspace{0.5mm}\\

\toprule
Barrier &
18.8 &
52.2 &
67.9 &
72.2 \\
Bicycle &
6.9  &
22.6 &
35.4 &
42.7 \\
Bus &
0.0 & 
3.6 &
23.2 &
37.3 \\
Car &
19.6 &
47.1 &
71.2 &
81.5 \\
Construction\_vehicle & 
0.0 &
1.9 &
13.5 &
25.0 \\
Motorcycle &
7.0 &
26.2 &
41.8 &
48.5 \\
Pedestrian & 
12.5 &
35.0 &
55.4 &
66.5 \\
Traffic\_cone &
31.7 &
53.3 &
64.8 &
71.3 \\
Trailer &
0.0 &
5.4 &
23.4 &
40.7 \\
Truck &
2.8 &
15.8 &
32.5 &
43.0 \\

% \bottomrule
\end{tabular}\\\vspace{0mm}
\caption{
\textbf{FCOS 3D detection results on the nuScenes~\cite{caesar2020nuscenes} test set:} detailed results for the AP metrics on all classes.}
\label{table:supp_nuscenes_per_class}
}
\end{table}

We present detailed results for all the object categories in Table~\ref{table:supp_nuscenes_per_class} (note that this complements Table 5 from the main paper). In addition, we present per-category metrics in terms of the three true-positive metrics used in nuScenes, i.e., Average Precision (AP), Average Translation Error (ATE), Average Scale Error (ASE) and Average Orientation Error (AOE) in Table~\ref{table:supp_nuscenes_all} (note that this complements the summary metrics presented in Table 4 of the main submission). We compare against the previous monocular state-of-the-art, MonoDis~\cite{simonelli2020disentangling}, and a widely used Lidar-based method, PointPillars~\cite{lang2019pointpillars}, in Table~\ref{table:supp_nuscenes_all}. We consistently outperform MonoDis  across most metrics, and even outperform PointPillars on average. Our method is particularly robust in detecting the long-tail of objects in rare categories.

\begin{table*}
\centering
{
\footnotesize
\setlength{\tabcolsep}{0.4em}
\rowcolors{2}{lightgray}{white}
\begin{tabular}{l|cccc|cccc|cccc}
\toprule
& \multicolumn{4}{c}{PointPillars~\cite{lang2019pointpillars}}& \multicolumn{4}{c}{MonoDis~\cite{simonelli2020demystifying}}& \multicolumn{4}{c}{FCOS-3D} \\

\multirow{-2}{*}{Category}& 
AP[\%]$\uparrow$ & ATE$\downarrow$ & ASE[1-IoU]$\downarrow$ & AOE[rad]$\downarrow$ &
AP[\%]$\uparrow$ & ATE$\downarrow$ & ASE[1-IoU]$\downarrow$ & AOE[rad]$\downarrow$ &
AP[\%]$\uparrow$ & ATE$\downarrow$ & ASE[1-IoU]$\downarrow$ & AOE[rad]$\downarrow$\vspace{0.5mm}\\

\midrule

Barrier & 39.0  & 0.71 & 0.30 & \textbf{0.08} & 50.0  & 0.54 & 0.28 & 0.22 &  \textbf{52.9} & \textbf{0.50} & \textbf{0.27} & 0.12 \\
Bicycle & 1.0  & \textbf{0.31} & 0.32 & \textbf{0.54} & 25.0 & 0.68 & \textbf{0.29} & 1.25  & \textbf{26.9} & 0.63 & 0.31 &  0.97  \\
Bus & \textbf{28.0}  & \textbf{0.56} & \textbf{0.20} & 0.25 & 15.0 & 0.85 & \textbf{0.20} & 0.12 & 16.0 & 0.93 &  \textbf{0.20} & \textbf{0.07} \\
Car & \textbf{68.0}  & \textbf{0.28} & 0.16 & 0.20 & 46.0 & 0.62 & \textbf{0.15} & 0.08 & 54.9 & 0.49 & \textbf{0.15} & \textbf{0.07} \\
Constr.Veh. & 4.0  & \textbf{0.89} & 0.49 & 1.26 &  6.0 & 1.02 & 0.41 & 1.05 & \textbf{10.1} & 0.97 & \textbf{0.39} & \textbf{0.94}  \\
Motorcycle & 27.0  & \textbf{0.36} & 0.29 & 0.79 &  30.0 & 0.70 & \textbf{0.24} & 0.57  & \textbf{30.9} &  0.64 & 0.25 & \textbf{0.48}  \\
Pedestrian & \textbf{60.0}  & \textbf{0.28} & 0.31 & \textbf{0.37} &  36.0 & 0.69 & \textbf{0.30} & 1.46  & 42.4 &  0.66 & 0.31 &  0.75  \\
Traffic Cone & 31.0  & \textbf{0.40} & 0.39 & - & 49.0 & 0.49 & \textbf{0.33} & – & \textbf{55.3} &  0.44 & 0.35 & -  \\
Trailer & \textbf{23.0}  & 0.89 & \textbf{0.20} & 0.83 &  16.0 & 1.03 & \textbf{0.20} & 0.78  & 17.4 & \textbf{0.88} & \textbf{0.20} & \textbf{0.72}  \\
Truck  & 23.0  & \textbf{0.49} & 0.23 & 0.18 &  21.0 & 0.79 & 0.20 & 0.10  & \textbf{23.5} & 0.68 & \textbf{0.19} & \textbf{0.07}  \\
\midrule
\textbf{Mean} & 31.0 & \textbf{0.52} & 0.29 & 0.50 & 30.0  & 0.74 & \textbf{0.26} & 0.62 & \textbf{33.0} & 0.68 &  \textbf{0.26} & \textbf{0.47} \\
\bottomrule
\end{tabular}\\\vspace{0mm}
\caption{\textbf{Results on nuScenes \emph{test}.} In addition to \emph{average precision}, FCOS-3D generally outperforms the previous best vision-based algorithm (\textbf{MonoDIS}) and a widely used Lidar-based algorithm (\textbf{PointPillars}) on multi-class metrics relevant to 3D detection. FCOS-3D is particularly robust in detecting rare objects, such as \emph{Construction Vehicle} and \emph{Traffic Cone}.}
%\textbf{FCOS 3D detailed detection results on the nuScenes~\cite{caesar2020nuscenes} test set.}}
\label{table:supp_nuscenes_all}
}
\end{table*}

\section{Cityscapes3D~\cite{gahlert2020cityscapes} results}
\label{sec:cityscapes}
In addition to KITTI3D~\cite{geiger2012we} and nuScenes~\cite{caesar2020nuscenes}, we also evaluate our method on the Cityscapes3D~\cite{gahlert2020cityscapes} benchmark. This novel dataset provides 3D object annotations using stereo depth, and thus provides an interesting alternative to other 3D datasets where objects are annotated in the lidar point cloud and then projected into the camera images. As done in Sec 5.2 of the main text  (cf. Fig.3 of the main submission), we measure the effect of performing additional pre-training using the "25K split" of the internal dataset. The only differences with the experiments on KITTI3D are that (i) we used class balanced sampling~\cite{Gupta_2019_CVPR} to address the imbalance between categories, and (ii) we used a new set of hyper-parameters in training ($0.008$ for learning rate, $32$ for batch size, $30000$ for training steps). We use the DLA-34\cite{yu2018deep}  backbone, and train the models on the \emph{train} subset, and evaluate on the \emph{val} subset of Cityscapes3D~\cite{gahlert2020cityscapes}. We report the average of $4$ models initialized with different random seeds during training. 

Our results are summarized in Table~\ref{table:supp_cityscapes_val_results}, where we report the same metrics used by nuScenes dataset in Table~\ref{table:supp_nuscenes_per_class}, i.e.,  average precision per class as well as the \emph{mean AP}. To the best of our knowledge, we are the first to evaluate metrics on this dataset, as no vision-only baselines exist. We argue that (i) the large gap in detection accuracy between nuScenes and CityScapes3D is mainly due to the difference in the size of training data ($\sim$1M vs. $\sim$3K), and (ii) the gap is significantly overcome by using parameters pre-trained on depth prediction ($14.38\%$ vs. $22.55\%$). 

% we compute and report in Table~\ref{table:supp_cityscapes_val_results} the Average Precision following the nuScenes~\cite{caesar2020nuscenes} format (i.e. we compute the AP over 4 distance thresholds, reporting the average), and note similar performance across the nuScenes and Cityscapes3D datasets. We also report the baseline performance in Table~\ref{table:supp_cityscapes_val_results}, noting as before a significant increase in performance when pre-training FCOS-3D with monocular depth estimation. 

% \input{tables/cityscapes_results}

\begin{table*}[!h]
\centering
{
\footnotesize
\setlength{\tabcolsep}{1em}
\rowcolors{2}{lightgray}{white}
\begin{tabular}{l|cccccc|c}
\toprule
& \multicolumn{7}{c}{mAP} \\

\multirow{-2}{*}{Method}& 
Car & Bicycle & Motorcycle & Truck & Train & Bus & Mean\vspace{0.5mm}\\
\toprule
FCOS-3D (COCO) & 
37.27 &
18.58 &
11.89 &
5.77  &
1.43  &
11.33 &
14.38 \\
FCOS-3D (25K) & 
\textbf{43.97}  & 
\textbf{34.66}  & 
\textbf{23.19}  & 
\textbf{11.27}  & 
\textbf{5.49}  & 
\textbf{16.70} & 
\textbf{22.55} \\  

% \bottomrule
\end{tabular}\\\vspace{0mm}
\caption{
\textbf{Effect of depth pre-training on Cityscapes 3D.} Starting from the initial set of parameters trained on 2D detection task using MS-COCO dataset \cite{lin2014microsoft}, we measure the effect of additional pre-training on supervised depth prediction. The second stage pre-training significantly improves accuracy on \emph{all} categories, yielding a relative $\textbf{56.8\%}$ gain in \emph{mean AP}. 
%\textbf{FCOS 3D detection results on the CityScapes3D~\cite{gahlert2020cityscapes} validation set.}
\label{table:supp_cityscapes_val_results}
}
}
\end{table*}

%\section{FCOS-3D ablative analysis (fine-tuning): detailed results}
\section{Fine-tuning DD3D with RoI-focused depth supervision}
\label{sec:fcos_ablative}

\begin{table*}
\centering
{
\footnotesize
\setlength{\tabcolsep}{0.35em}
\rowcolors{2}{lightgray}{white}
\begin{tabular}{l|ccc|ccc||ccc|ccc||ccc|ccc}
\toprule
& \multicolumn{6}{c}{Car} & \multicolumn{6}{c}{Pedestrian} & \multicolumn{6}{c}{Cyclist} \\
& \multicolumn{3}{c}{BEV AP} & \multicolumn{3}{c}{3D AP} & \multicolumn{3}{c}{BEV AP} & \multicolumn{3}{c}{3D AP} & \multicolumn{3}{c}{BEV AP} & \multicolumn{3}{c}{3D AP} \\ 
\multirow{-3}{*}{Method}& 
Easy & Mod & Hard & Easy & Mod & Hard & Easy & Mod & Hard & Easy & Mod & Hard & Easy & Mod & Hard & Easy & Mod & Hard\vspace{0.5mm} \\
\toprule
FCOS-3D & 
33.23 & 25.82 & 21.75 & 24.01 & 18.20 & 14.85 &
12.58 & 9.93&  \textbf{7.88} & 9.76 & 7.64 & 5.80 & 
\textbf{7.58} & \textbf{4.36} & \textbf{3.64} & \textbf{6.60} & \textbf{3.76} & \textbf{2.98} \\

FCOS-3D Multi-task & 
\textbf{34.62} & \textbf{26.27} & \textbf{22.12} & \textbf{24.12} & \textbf{18.21} & \textbf{14.89} &
\textbf{12.79} & \textbf{10.09} &  7.77 & \textbf{10.51} & \textbf{8.18} & \textbf{6.05} & 
6.58 & 3.91& 3.17 & 5.14 & 2.99 & 2.41 \\

\bottomrule
\end{tabular}\\\vspace{0mm}
\caption{
\textbf{Supervised depth prediction as auxiliary task during fine-tuning.} We present the full experimental results showing the effect of using region-of-interest (RoI) focused depth supervision as an auxiliary task during fine-tuning for 3D detection. This complements Table 8 of the main paper by including "Easy" and "Hard" metrics of KITTI-3D benchmark.
%\textbf{Ablative analysis on different FCOS-3D fine-tuning strategies on the target dataset.} We present detailed results using the BeV and 3DAP metrics, complementing the results from Table 8 in the main submission. The metrics are computed on the KITTI3D~\cite{geiger2012we} validation split.
}
\label{table:supp_detailed_multi_task}
}
\end{table*}

In Table 8 of the main submission, we present an abridged version of the full KITTI benchmark results showing the effect of using auxiliary depth loss computed on region-of-interest (RoI), while fine-tuning DD3D for 3D detection. In Table~\ref{table:supp_detailed_multi_task}, we present the full benchmark results that include "Easy" and "Hard" metrics for all object categories. The conclusion remains unchanged: additional depth fine-tuning on the target domain marginally improves performance on some classes, while decreasing performance on others. That is, fine-tuning depth prediction on target domain yields only marginal gain over the pre-training using large-scale image-Lidar data. Note that this is in contrast to Pseudo-Lidar methods, which require a specialized fine-tuning step for the detection networks in the target domain.

% To recapitulate, we explored the potential of using Lidar point-cloud in the target domain (in this case KITTI scenes) by adding a loss measuring the mean L1-distance of predicted and ground-truth depth to the 3D detection losses of FCOS-3D. 
%We present detailed 3D detection results in Table~\ref{table:supp_detailed_multi_task} (note that these results complement the results presented in Table 8 of the main submission). The numbers indicate that additional depth fine-tuning on the target domain marginally improves performance on some classes, while decreasing performance on others. Note that this is in contrast to Pseudo-Lidar methods, which require a specialized fine-tuning step for the detection networks in the target domain.

\section{Details of depth pre-training}
\label{sec:pretraining}
We provide the full details of the training schedule used for supervised monocular depth pre-training of both DD3D and PackNet.

\noindent\textbf{DD3D.} For all supervised depth pre-training splits (1K, 5K, 10K, 25K), we use L1 loss between predicted depth and projective ground-truth depth, and $256$ as batch size. The size of input images (and projected depth map) is 1600 $\times$ 900, and we resize them into 910 $\times$ 512. When resizing the depth maps, we perserved the sparse depth values by assigning all non-zero depth values to the nearest-neighbor pixel in the resized image space (Note that this is different from naive nearest-neighbor , where the target depth value is assigned zero, if the nearest-neighbor pixel in the original image does not have depth value.) We observed the training converges after 15 epochs. We use momentum optimizer with $\beta = 0.99$.  

\noindent\textbf{PackNet.} We train the monocular depth estimation network PackNet~\cite{guizilini20203d} on each pre-training split. In each case we use a batch size of $4$, constant learning rate of $5e^{-5}$, input resolution of $640\times 480$ and the Adam~\cite{loshchilov2017decoupled} optimizer with $\beta_1=0.9$ and $\beta_2=0.999$. We train until convergence on each split (1K, 5K, 10K, 25K), i.e. until the depth metrics computed (see Table~\ref{table:supp_pl_data_vs_det}) stabilize. Specifically, for each split we trained for 20 epochs, with the exception of 1K where we noticed convergence after 10 training epochs. 

% The training splits contain an increasing number of images, as follows: 1K: $10^6$ images, 5K: $5\cdot 10^6$ images, 10K: $10 \cdot 10^6$ images, 25K: $25 \cdot 10^6$ images. For each we train until convergence, i.e. until the depth metrics computed (see Table~\ref{table:supp_pl_data_vs_det}) stabilize. 

\section{Pseudo-Lidar 3D confidence head}
\label{sec:pl_detection_head}

Our PL 3D detector is based on~\cite{ma2020rethinking}, and outputs 3D bounding boxes with 3 heads, separated based on distance (i.e. near, medium and far). Following~\cite{simonelli2019disentangling,simonelli2020demystifying} we modify each head to output a 3D confidence, trained through the 3D bounding box loss as described in the main submission. Specifically, each 3D box estimation head consists of 3 fully connected layers with dimensions $512 \longrightarrow 512 \longrightarrow 256 \longrightarrow  \left(\delta,\gamma\right)$, where $\delta$ denotes the bounding box parameters as described in~\cite{ma2020rethinking}, and $\gamma$ denotes the 3D bounding box confidence.

\section{DD3D architecture details}
\label{sec:fcos_architecture}

\noindent\textbf{FPN} As described in \cite{lin2016fpn}, a feature pyramid network (FPN) is composed of \emph{bottom-up} network which is a feed-forward CNN that computes feature maps with a scaling step of 2, and a \emph{top-down} network with lateral connections that recovers high-resolution features from low-resolution ones. We use two types of bottom-up network, DLA-34 \cite{yu2018deep} and V2-99 \cite{lee2019centermask}. Both FPNs yield 5 levels of feature maps. For DLA-34, the FPN features are first computed across three levels (with step size of 8, 16, and 32) using the standard FPN computation \cite{lin2016fpn}, and then two lower resolution features (with step size of 64, 128) are computed by stacking two $3\times3$ 2D convolution with stride equals to 2 on top of highest level features of FPN (See Fig 2 of the main paper for an illustration). For V2-99, the bottom-up network (and therefore the standard FPN features) by default produces 4 levels of features (step size = 4, 8, 16, and 32). We create an additional level of features by adding one $3\times3$ 2D convolution. Note that the final resolution of FPN features derived from DLA-34 and V2-99 network is different, DLA-34 computes features with step sizes equal to 8, 16, 32, 64, and 128, while V2-99 computes the ones that are equal to 4, 8, 16, 32, and 64. 

\noindent\textbf{2D detection head} 
For 2D detector, we closely follow the decoder architecture and loss formulation of the original FCOS~\cite{tian2019fcos}.
In addition, we adopt the recent changes introduced in the updated version~\cite{fcos-arxiv} in positive sampling approach.
%The only difference from the original FCOS \cite{tian2019fcos} is the recently introduced matching strategy, i.e. how to match CNN features to each object (or its 2D bounding box).
Recently, the authors of~\cite{tian2019fcos} showed that center-based positive sampling, as suggested in~\cite{zhou2019objects}, yields additional gain in 2D detection accuracy.
%That is, instead of using all CNN features that falls within the 2D bounding box, one uses only the features that are close to the center of the bounding box. We adopt this matching strategy for matching. 
Under the new center-based approach, only the center-portion of the gound truth bounding box are used to assign positive samples in $\mathcal{L}_{reg}$ (Eq. 3); see~\cite{fcos-arxiv} for additional details.

\section{The impact of data on depth and 3D detection}
\label{sec:supp_data_vs_3d_det}

We evaluate depth quality against the 3D detection accuracy of the PL detector, with results shown in Fig.~\ref{fig:3d_vs_depth}. Our results indicate an almost perfect linear relationship between depth quality as measured by the \textit{abs\_rel} metric and 3D detection accuracy for our PL-based detector.

\begin{figure}[h]
    \includegraphics[width=0.99\columnwidth,trim={0mm 0mm 0mm 0mm},clip]{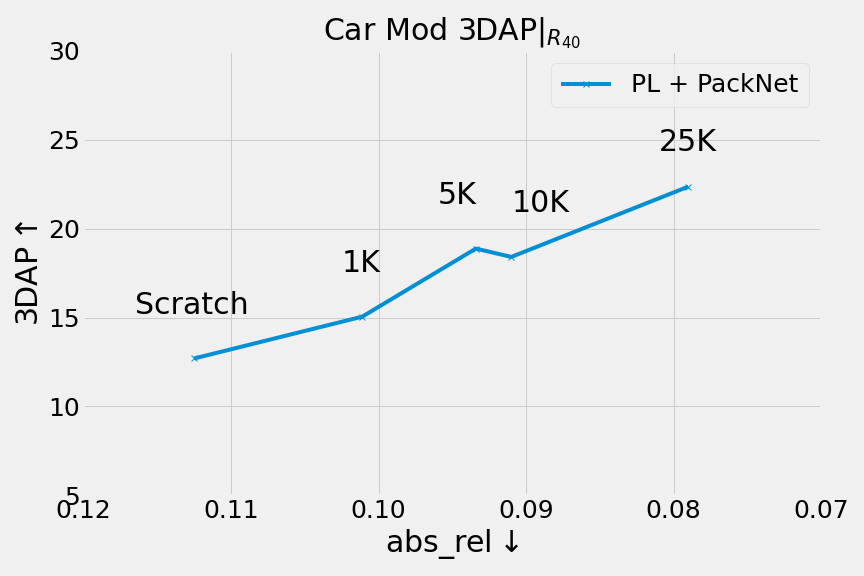}
    \caption{\textbf{We evaluate depth performance (abs\_rel) against PL 3D detection performance (Car 3DAP$|_{R_{40}}$) at each pre-training step.} Our results indicate an almost perfect linear relationship between depth quality and 3D detection accuracy. All results are computed on the KITTI3D validation split.}
    \label{fig:3d_vs_depth}
\end{figure}

\section{Qualitative results}
\label{sec:qualitative}

We present additional qualitative results on Cityscapes3D~\cite{gahlert2020cityscapes} in Figure~\ref{fig:supp_results_qualitative_cs}, KITTI~\cite{geiger2012we} in Figure~\ref{fig:supp_results_qualitative} and nuScenes~\cite{caesar2020nuscenes} in Figure~\ref{fig:supp_results_qualitative_nusc}. To generate the qualitative results we apply non-maxima suppression (NMS) with 0.3 as threshold on intersection-over-union (IoU). We show detected bounding boxes with confidence higher or equal to 0.4. We also refer readers to the supplementary video that shows the DD3D output on the nuScenes \emph{val} images, which are videos sampled at 2Hz, along with a high-level overview of our paper.
\begin{figure*}
\vspace{-2mm}
\centering
% [trim=left bottom right top, clip]

\subfloat{
\includegraphics[width=0.45\linewidth]{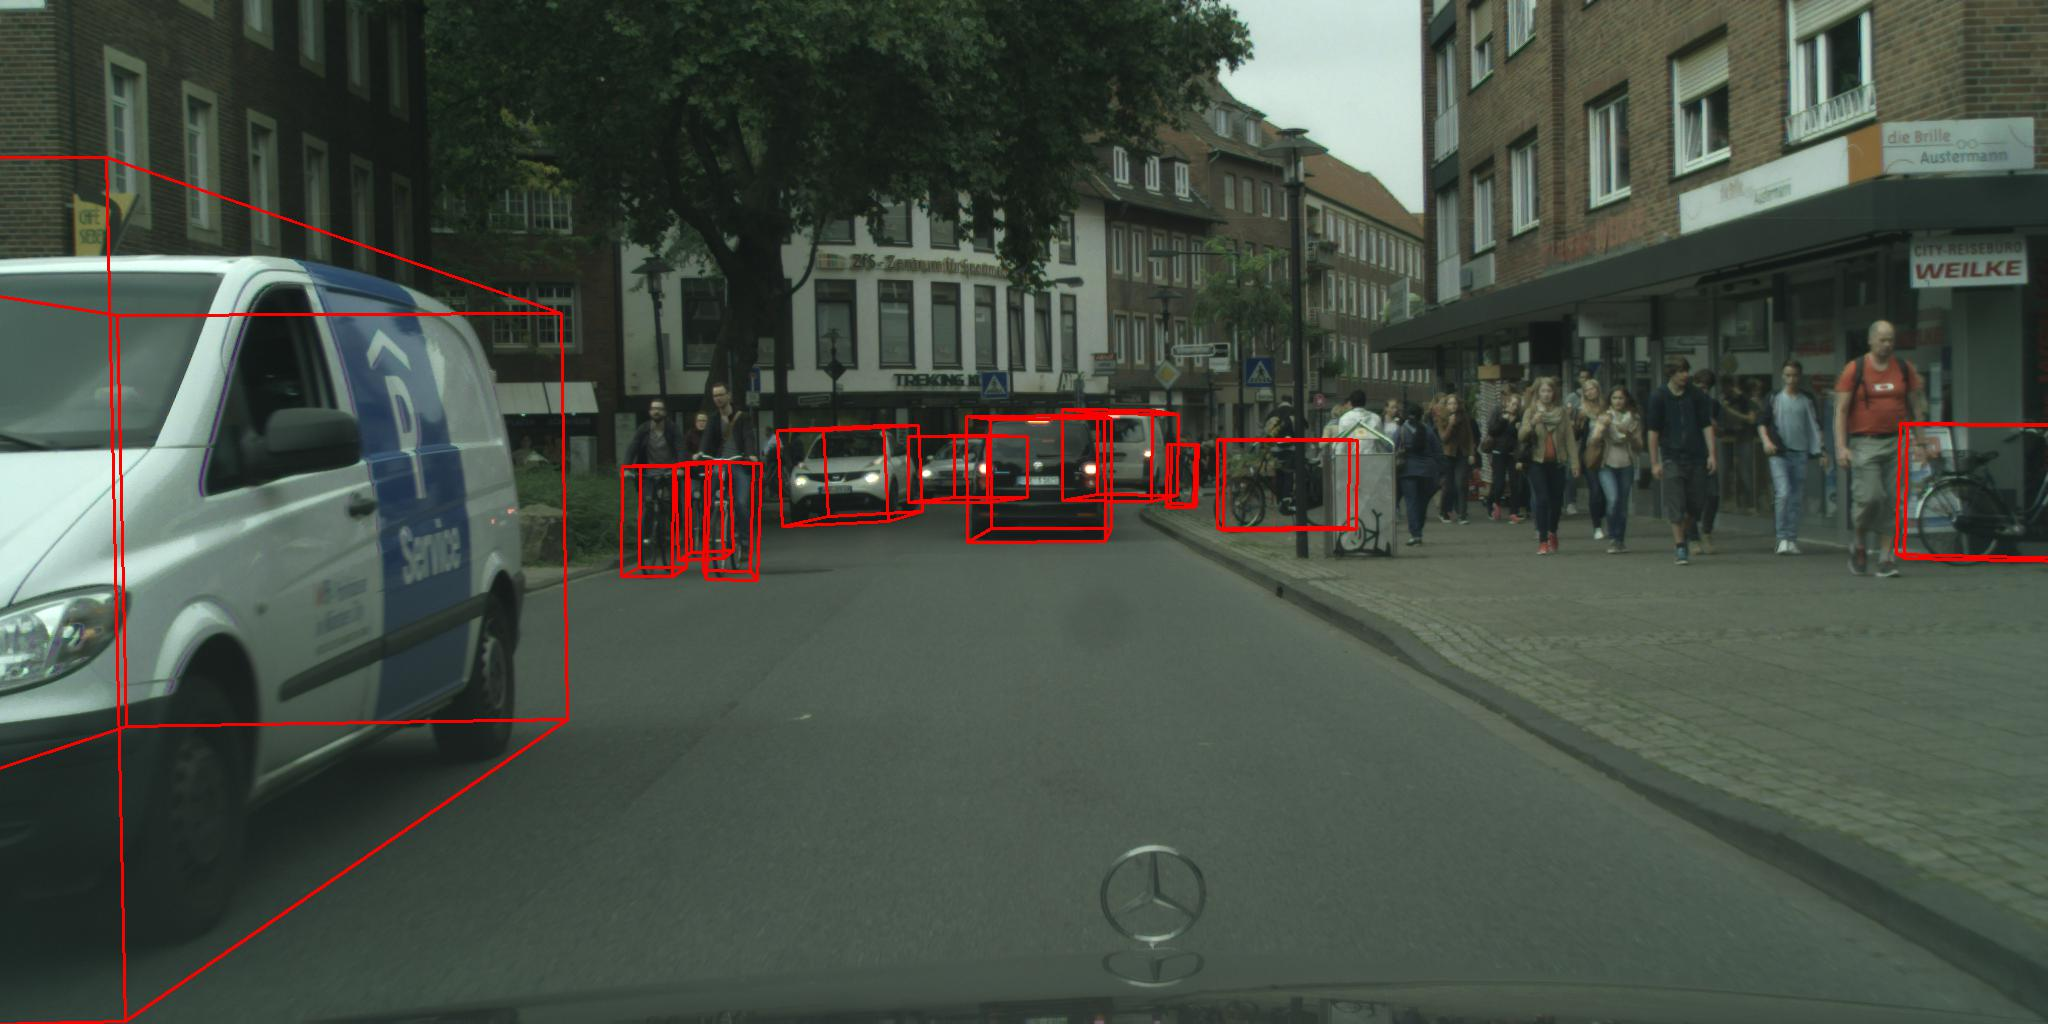}
\includegraphics[trim=0 0 0 0,clip,width=0.45\linewidth]{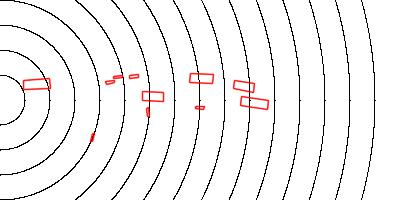}
} \\ 
\subfloat{
\includegraphics[width=0.45\linewidth]{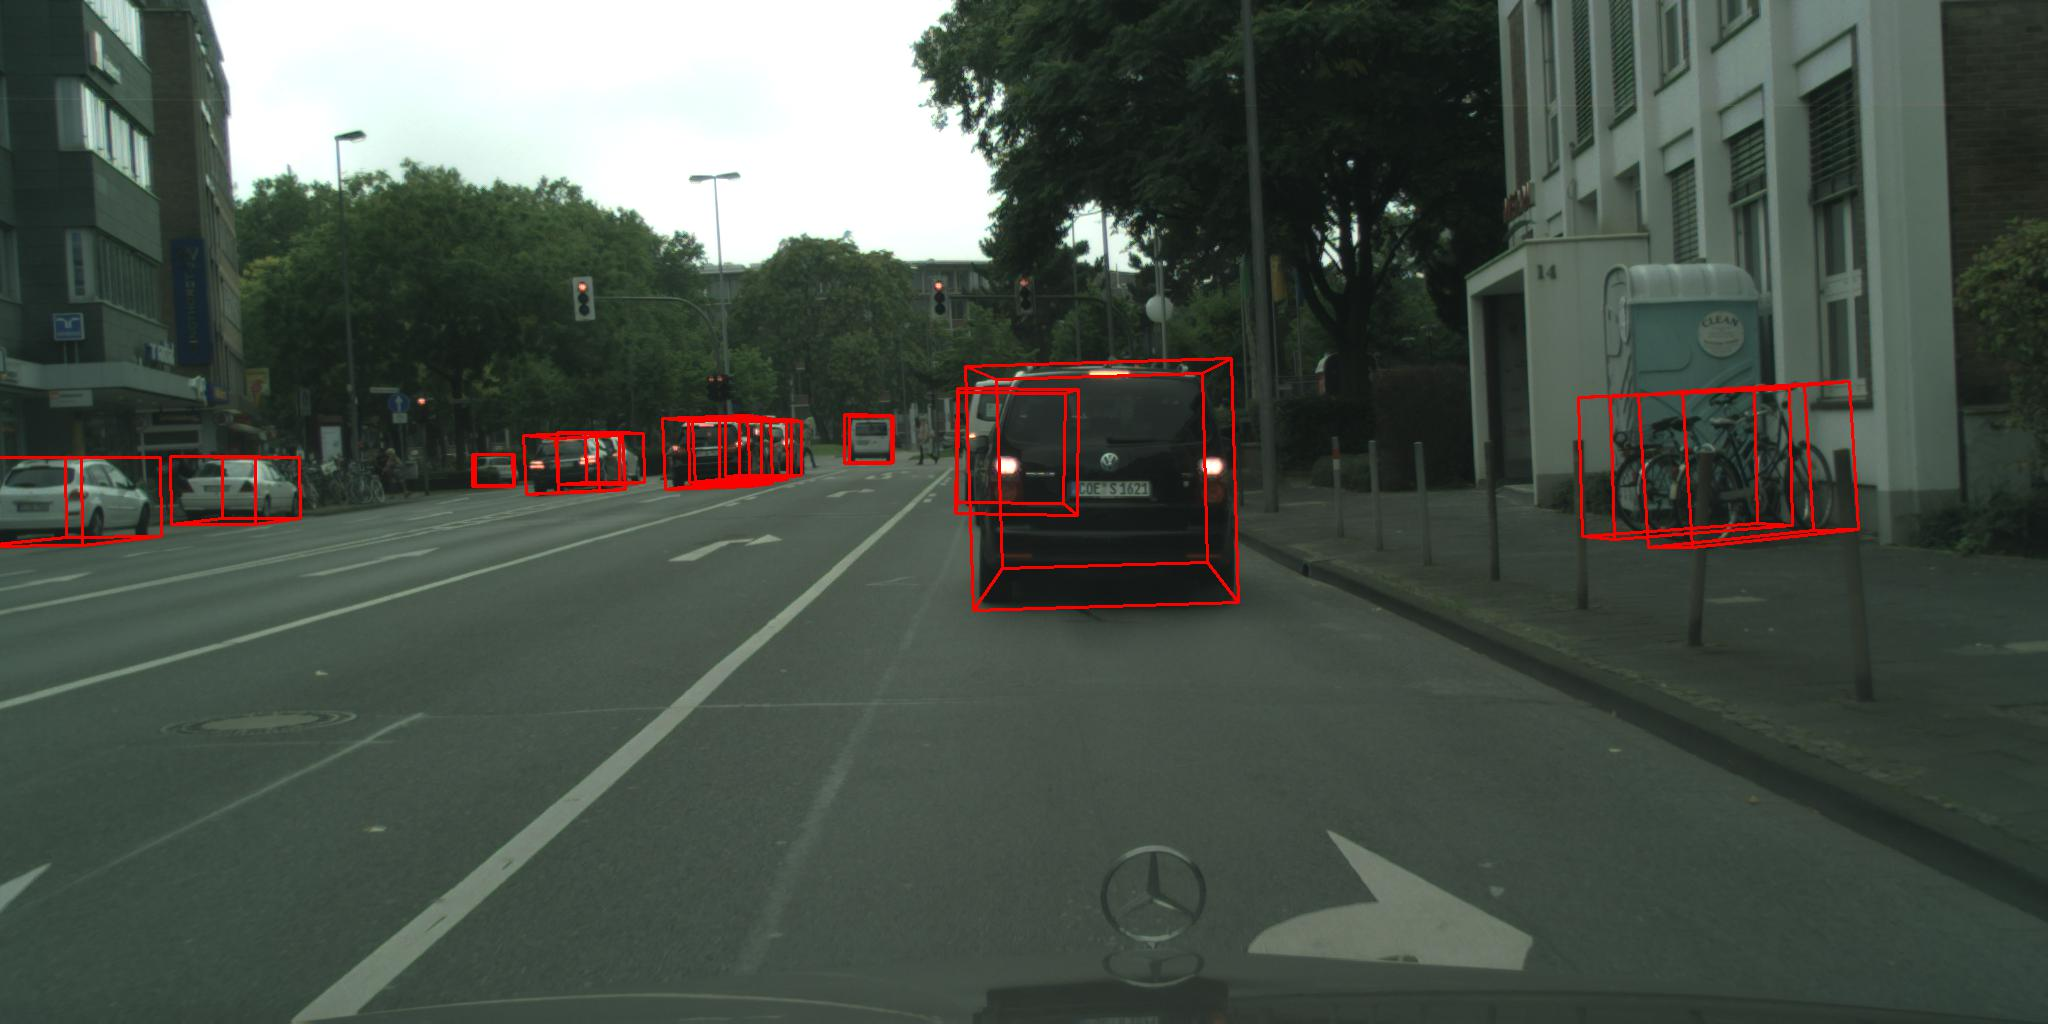}
\includegraphics[trim=0 0 0 0,clip,width=0.45\linewidth]{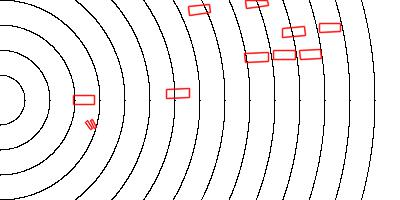}
} \\

\vspace*{-2mm}
\caption{
\textbf{Qualitative results of DD3D applied on the Cityscapes3D~\cite{gahlert2020cityscapes} \emph{val}}. Cityscapes 3D contains bounding boxes of 6 types of vehicles (no pedestrian). In the bird-eye-view visualization (\textbf{left}), the concentric circles are $5$m apart. 
}
\label{fig:supp_results_qualitative_cs}
\end{figure*}

\begin{figure*}
\vspace{-2mm}
\centering
% [trim=left bottom right top, clip]
\subfloat{
\includegraphics[width=0.65\linewidth]{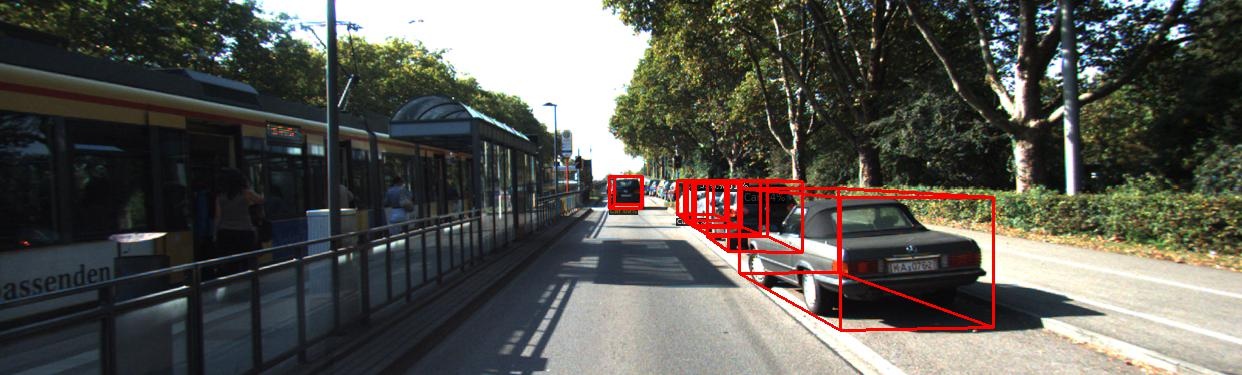}
\includegraphics[width=0.25\linewidth]{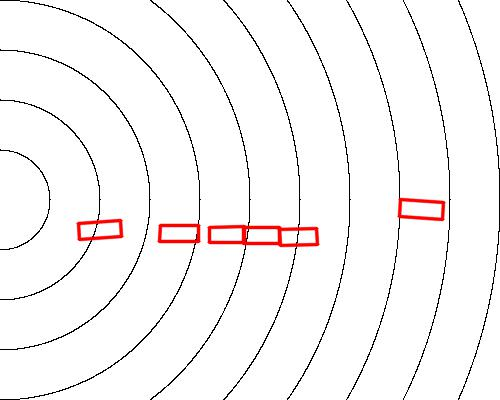}
} \\ 
\subfloat{
\includegraphics[width=0.65\linewidth]{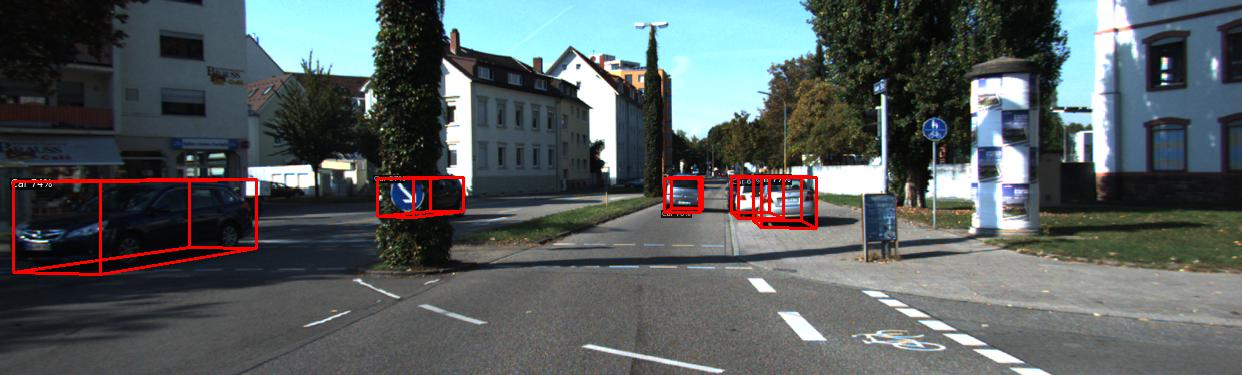}
\includegraphics[width=0.25\linewidth]{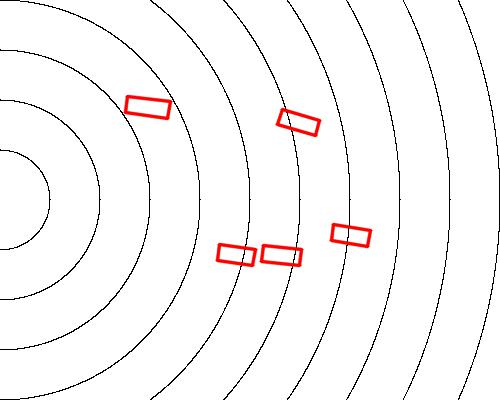}
}\\

\vspace*{-2mm}
\caption{
\textbf{Qualitative results of FCOS-3D applied on the KITTI3D ~\cite{geiger2012we}.} It can detect highly occluded cars up to 75m, achieving state-of-the-art vision-based method on KITTI \emph{test}.}
\label{fig:supp_results_qualitative}
\end{figure*}

\begin{figure*}
\vspace{-2mm}
\centering
% [trim=left bottom right top, clip]

\subfloat{
\includegraphics[width=0.49\linewidth]{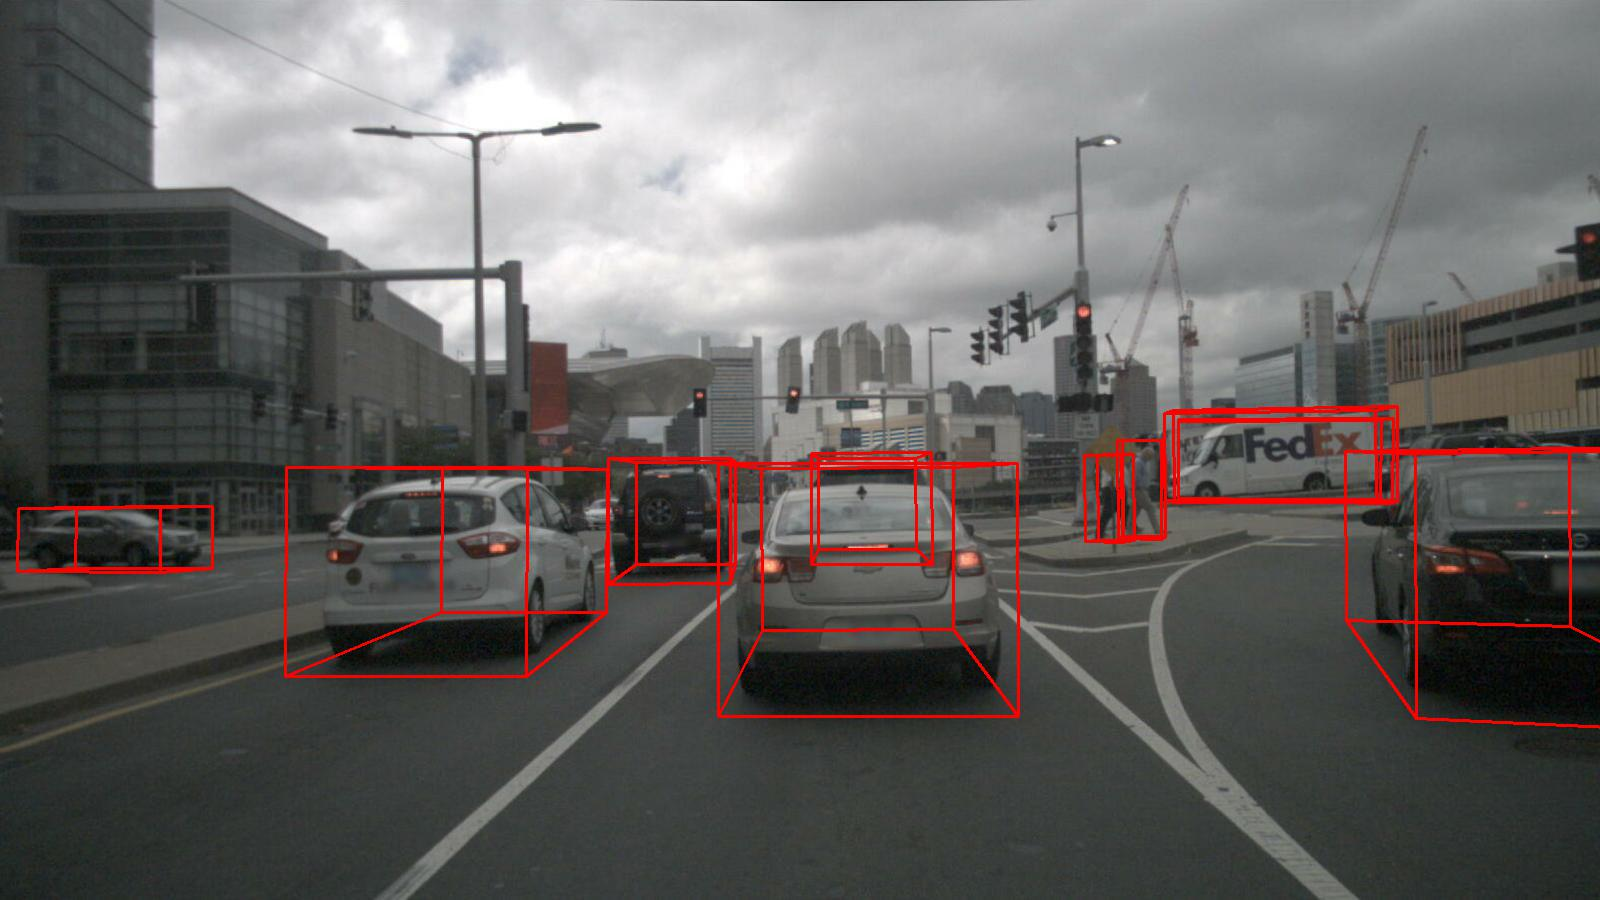}
\includegraphics[trim=0 0 120 0,clip,width=0.38\linewidth]{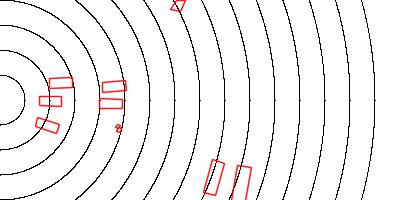}
} \\ 
\subfloat{
\includegraphics[width=0.49\linewidth]{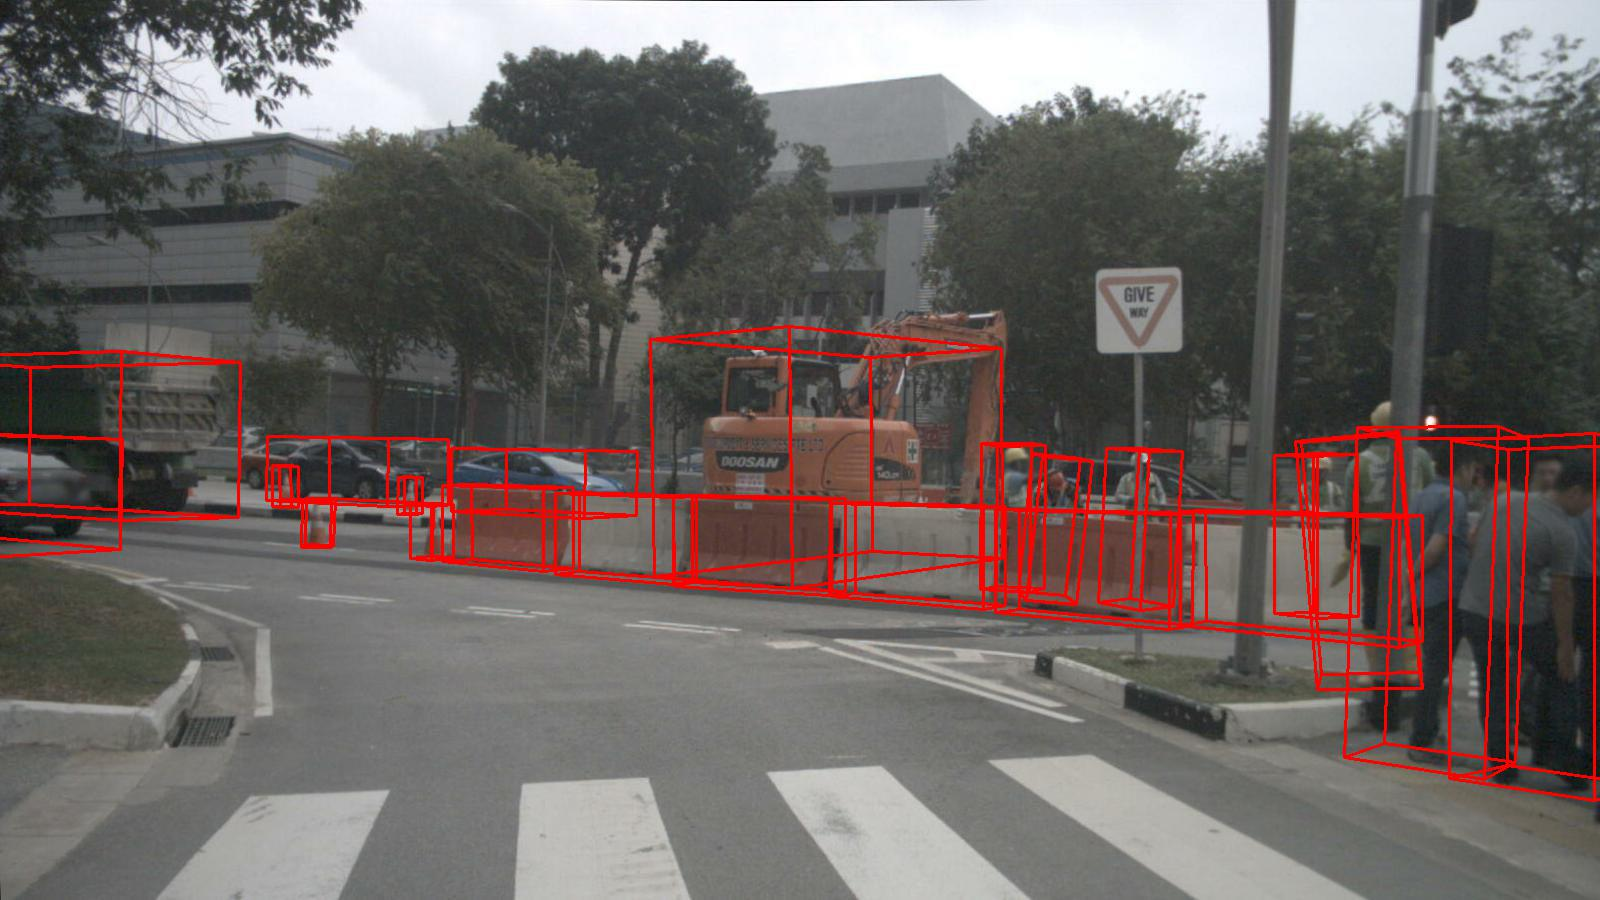}
\includegraphics[trim=0 0 120 0,clip,width=0.38\linewidth]{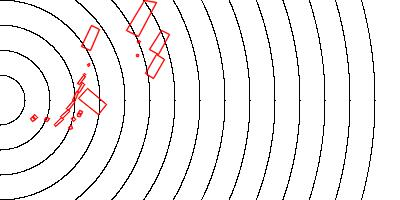}
} 
\vspace*{-2mm}
\caption{
\textbf{Qualitative results of DD3D applied on the nuScenes~\cite{caesar2020nuscenes} \emph{val}}. nuScenes contains bounding boxes of 10 object categories, including "Pedestrian", "Barrier" and "Traffic Cone", and "Construction Vehicle" (all shown above). We only show the results from front camera. 
}
\label{fig:supp_results_qualitative_nusc}
\end{figure*}
